# Supplementary material for: Learning Cross-Scale Visual Representations for Real-Time Image Geo-Localization
Source: arXiv:2109.04087 source file (2022-05-14)
Supplement: Supplementary file 1 [file appendix.tex]

asdfasdfasdfasdfdas
